# Supplementary material for: d+id' Chiral Superconductivity in Bilayer Silicene
Source: arXiv:1208.5596 source file (2013-08-11)
Supplement: Supplementary file 1 [file Supplementary_Material.pdf]

# *d+id'* Chiral Superconductivity in Bilayer Silicene

Feng Liu, Cheng-Cheng Liu, Kehui Wu, Fan Yang, and Yugui Yao

## I. POSSIBLE STRUCTURES

Due to the weakened $\pi-$bond between adjacent Si-atoms, the silicene layer possesses a low-buckled non-planar structure, which is different from that of the graphene. In this structure, a silicene layer is divided into two halves, i.e. the top and bottom, with each occupying one of the two sublattices (A and B) of the original honeycomb lattice. As a result of this non-planar structure of a silicene layer, there can be four possible stacking ways between the two layers in the bilayer silicene (BLS), i.e. the AA bottom-bottom (AA-bb), the AA bottom-top (AA-bt), the AB bottom-top (AB-bt), and the AB bottom-bottom (AB-bb). The geometries and phonon spectra corresponding to these four structures are shown in Fig.1, and the corresponding optimized energies and parameters are listed in Table I

Note that the configurations are fully relaxed until the force on every atom is less than $10^{-3}$ eV/$\AA$. $33 \times 33 \times 1$ k points are sampled in Brillouin zone for the self consistent field cycle with energy tolerance of $1.0^{-6}$ eV. To perform precise calculation, a 400 eV energy cutoff for the plane-wave basis and a vacuum layer of 20 $\AA$ are set. For phonon spectrum calculations, $3\times3\times1$ supercell and $7 \times 7 \times 1$ k points grid in Brillouin zone are used.

From Fig.1, it's clear that the four possible structures of the system possess different symmetries. The AA-bb and AB-bt structures shown in Fig.1a and Fig.1c possess the $D_{3d}$ symmetry, while

TABLE I: **Optimized energies and geometric parameters corresponding to the four possible structures of the BLS.** The second column gives the energy per unit cell. In the third column, the first and second number provide the bond-lengths of the nearest neighbor intra-layer and inter-layer valence bonds respectively. The final column is the angle between these two kinds of valence bonds. Note that in the AB-bb structure, the exchange symmetry between the upper and lower layers has been broken, as reflected in the different bond-lengths and bond-angles for the two layers.

| Structure | Energy(eV) | Bond-length(Å) | Bond-Angle |
|---|---|---|---|
| AA-bb | -19.14 | 2.28, 5.12 | $101.52^o$ |
| AA-bt | -19.51 | 2.32, 2.46 | $106.48^o$ |
| AB-bt | -19.65 | 2.32, 2.53 | $106.60^o$ |
| AB-bb | -19.30 | 2.31(2.34), 2.92 | $107.77^o(109.53^o)$ |

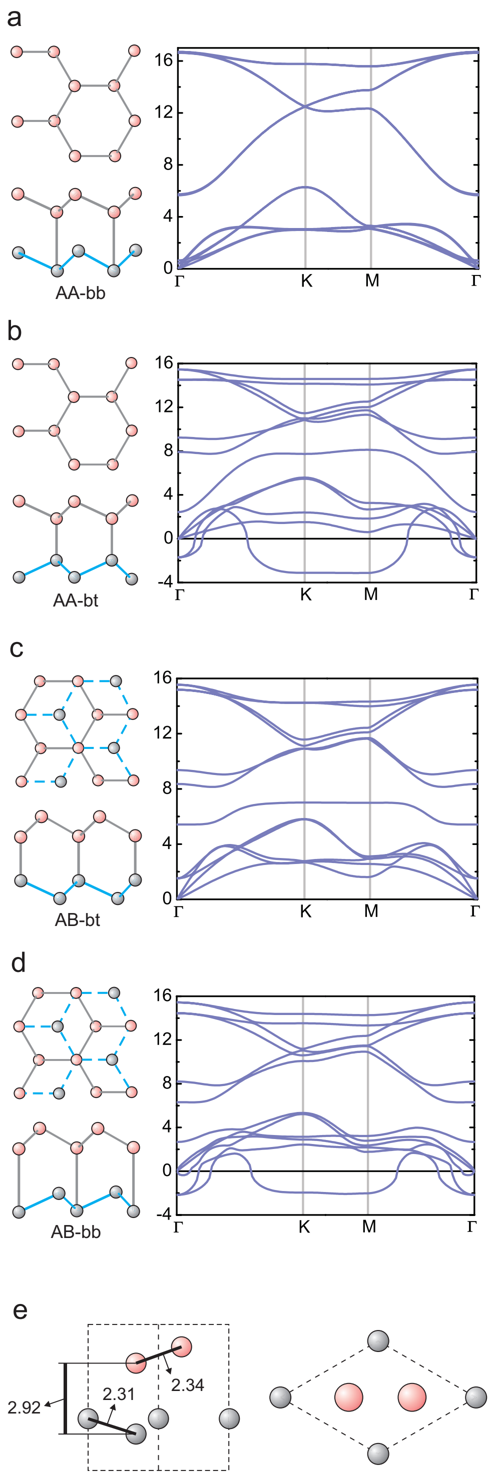


FIG. 1: **Geometries and phonon spectra corresponding to the four possible structures of the BLS. a-d**, Geometries and phonon spectra for the AA-bb (a), AA-bt (b), AB-bt (c) and AB-bb (d) structures of the BLS. In each show, the upper left is the top view, the lower left is the side view and the right is the phonon spectrum corresponding to each structure. Note that negative frequencies shown actually represent imaginary values obtained and thus imply structure instability. **e**, More details for the configuration of the AB-bb structure, where one finds the breaking of the exchange symmetry between the two layers in this structure.

the point group of the AA-bt structure shown in Fig.1b is $D_{3h}$. The AB-bb structure shown in Fig.1d has the smallest symmetry group among the four, i.e. $C_{3v}$, since the different bond-lengths and bond-angles between the two layers shown in Fig.1e and Table I. From the phonon spectra corresponding to these structures, one finds that Fig.1b and Fig.1d are unstable toward structure reconfiguration because of the imaginary frequencies obtained, leaving only the two symmetric structures shown in Fig.1a and Fig.1c as possible candidates of realizable structure.

The AA-bb structure shown in Fig.1a can be considered as a simple analogy to the AA-stacked BLG which consists of two graphene layers weakly coupled through the van der Waals interaction. Consequently, one finds from Table I that the inter-layer bond-length corresponding to this structure is extremely large. This structure is energetically worst although it is locally stable. The AA-bt structure shown in Fig.1b is just the one studied in Ref [1]. Although the energy of this structure is somewhat favorable, it is locally unstable. The structure Fig.1d is not energetically favored either. The optimal structure of the BLS should be the AB-bt structure shown in Fig.1c which is focused in the present work as it is not only energetically most favored but also locally stable. The bond-angle of this structure is $106.60^o$, very near to that of the $sp^3$ hybridization, i.e $109.47^o$. The inter-layer bond-length is 2.53 $\mathring{A}$, near to the 2.32 $\mathring{A}$ of the intra-layer bond-length. Combination of the two features describes an $sp^3$-like orbital hybridization rather than a planar $sp^2$-like one.

The band structures corresponding to the above four crystal structures are shown in Fig.2. In the AA-bb band structure shown in Fig.2a, two crossings slightly deviating from each K point are present at the Fermi level, which leads to a semi-metal ground state. This state is not favored by energy, as illustrated above. The AA-bt band structure shown in Fig.2b has been studied in Ref [1]. The two crossings locating on the $\Gamma-$M and $\Gamma-$K lines are present around the Fermi level. However, our FP calculations reveal that this state is neither energetically most favored nor stable. The AB-bt band structure shown in Fig.2c is the finally optimized one. Large band overlap and asymmetric band crossings are present in this band structure, which leads to the pocket Fermi surface (FS) structure shown in Fig.2e. The six-folded rotation symmetry of the FS is required by the $D_{3d}$ and time reversal symmetry of the system. From this band structure, one obtains an intrinsically metallic ground state with finite DOS at the Fermi level, which opens the door to formation of SC. The AB-bb band structure shown in Fig.2d is somewhat similar with Fig.2c in that it also possesses band overlap. However, it is energetically unfavored. Note that since the experimentally measured lattice constant is about 6.4 $\mathring{A}$ for the $\sqrt{3}\times\sqrt{3}$ reconstructed second layer silicene on Ag(111)[2], which can be corresponded to 3.8 $\mathring{A}$ per unit cell, we only discuss the

TABLE II: **TB parameters fitted for the BLS under different strain conditions.** The unit is eV.

| Strain | $t_n$ | $t$ | $t_2$ | $t_3$ | $\Delta$ |
|---|---|---|---|---|---|
| 0.00 | 1.130 | 2.025 | 0.152 | 0.616 | -0.069 |
| 0.01 | 1.079 | 1.974 | 0.159 | 0.595 | -0.073 |
| 0.02 | 1.045 | 1.947 | 0.162 | 0.585 | -0.077 |
| 0.03 | 1.012 | 1.924 | 0.163 | 0.573 | -0.082 |
| 0.04 | 0.980 | 1.904 | 0.162 | 0.562 | -0.088 |
| 0.05 | 0.948 | 1.878 | 0.161 | 0.551 | -0.092 |
| 0.06 | 0.912 | 1.844 | 0.158 | 0.541 | -0.100 |

configurations with close lattice constants. However, if we give up this restriction, there are some other stable configurations, for example the one studied by Ref [3], and in subsequent research work, we will get into this aspect in more detail.

It's important that the biaxial strain exerted on the system has obvious influence on the low energy band structure of the system. In the following Table II, we list the tight-binding (TB) parameters fitted for each strain up to 0.06, under which the symmetry and FS topology of the system are kept.

## II. FOUR-ORBITAL RPA

In this part, we provide details of the four-orbital random phase approximation (RPA) approach [4–9] adopted in the study of the above Hubbard-model (formula (2) in the main text).

### A. RPA susceptibility

Let's define,

$$\chi^{(0)l_1,l_2}_{l_3,l_4}(\mathbf{q},\tau) \equiv \frac{1}{N}\sum_{\mathbf{k_1},\mathbf{k_2}} \left\langle T_\tau c^\dagger_{l_1}(\mathbf{k_1},\tau) c_{l_2}(\mathbf{k_1}+\mathbf{q},\tau) c^+_{l_3}(\mathbf{k_2}+\mathbf{q},0) c_{l_4}(\mathbf{k_2},0)\right\rangle_0 \quad (1)$$

to be the free susceptibility for $U=0$, with $l_i$ $(i=1,\cdots,4)$ denoting orbital index. The explicit formulism of $\chi^{(0)}$ in the momentum-frequency space is,

$$\chi^{(0)l_1,l_2}_{l_3,l_4}(\mathbf{q},i\omega_n) = \frac{1}{N}\sum_{\mathbf{k},\alpha,\beta}\xi^{\alpha}_{l_4}(\mathbf{k})\xi^{\alpha,*}_{l_1}(\mathbf{k})\xi^{\beta}_{l_2}(\mathbf{k}+\mathbf{q})\xi^{\beta,*}_{l_3}(\mathbf{k}+\mathbf{q})\frac{n_F(\varepsilon^{\beta}_{\mathbf{k}+\mathbf{q}})-n_F(\varepsilon^{\alpha}_{\mathbf{k}})}{i\omega_n+\varepsilon^{\alpha}_{\mathbf{k}}-\varepsilon^{\beta}_{\mathbf{k}+\mathbf{q}}}, \tag{2}$$

where $\alpha,\beta = 1,...,4$ are band indices, $\varepsilon^{\alpha}_{\mathbf{k}}$ and $\xi^{\alpha}_{l}(\mathbf{k})$ are the $\alpha-$th eigenvalue and eigenvector of the $H(\mathbf{k})$ matrix (equation (1) in the main text) respectively and $n_F$ is the Fermi-Dirac distribution function.

When interaction turns on, we define the spin ($\chi^{(s)}$) and charge ($\chi^{(c)}$) susceptibility as follow,

$$\begin{aligned}
\chi^{(c)l_1,l_2}_{l_3,l_4}(\mathbf{q},\tau) &\equiv \frac{1}{2N}\sum_{\mathbf{k_1},\mathbf{k_2},\sigma_1,\sigma_2}\left\langle T_\tau C^{\dagger}_{l_1,\sigma_1}(\mathbf{k_1},\tau)C_{l_2,\sigma_1}(\mathbf{k_1}+\mathbf{q},\tau)C^{+}_{l_3,\sigma_2}(\mathbf{k_2}+\mathbf{q},0)C_{l_4,\sigma_2}(\mathbf{k_2},0)\right\rangle, \\
\chi^{(s^z)l_1,l_2}_{l_3,l_4}(\mathbf{q},\tau) &\equiv \frac{1}{2N}\sum_{\mathbf{k_1},\mathbf{k_2},\sigma_1,\sigma_2}\sigma_1\sigma_2\left\langle T_\tau C^{\dagger}_{l_1,\sigma_1}(\mathbf{k_1},\tau)C_{l_2,\sigma_1}(\mathbf{k_1}+\mathbf{q},\tau)C^{+}_{l_3,\sigma_2}(\mathbf{k_2}+\mathbf{q},0)C_{l_4,\sigma_2}(\mathbf{k_2},0)\right\rangle, \\
\chi^{(s^{+-})l_1,l_2}_{l_3,l_4}(\mathbf{q},\tau) &\equiv \frac{1}{N}\sum_{\mathbf{k_1},\mathbf{k_2}}\left\langle T_\tau C^{\dagger}_{l_1\uparrow}(\mathbf{k_1},\tau)C_{l_2\downarrow}(\mathbf{k_1}+\mathbf{q},\tau)C^{+}_{l_3\downarrow}(\mathbf{k_2}+\mathbf{q},0)C_{l_4\uparrow}(\mathbf{k_2},0)\right\rangle, \\
\chi^{(s^{-+})l_1,l_2}_{l_3,l_4}(\mathbf{q},\tau) &\equiv \frac{1}{N}\sum_{\mathbf{k_1},\mathbf{k_2}}\left\langle T_\tau C^{\dagger}_{l_1\downarrow}(\mathbf{k_1},\tau)C_{l_2\uparrow}(\mathbf{k_1}+\mathbf{q},\tau)C^{+}_{l_3\uparrow}(\mathbf{k_2}+\mathbf{q},0)C_{l_4\downarrow}(\mathbf{k_2},0)\right\rangle.
\end{aligned} \tag{3}$$

Note that in non-magnetic state we have $\chi^{(s^z)} = \chi^{(s^{+-})} = \chi^{(s^{-+})} \equiv \chi^{(s)}$, and when $U = 0$ we have $\chi^{(c)} = \chi^{(s)} = \chi^{(0)}$.

In the RPA level, the spin/charge susceptibility for the Hubbard-model (formula (2) in the main text) is,

$$\begin{aligned}
\chi^{(s)}(\mathbf{q},i\nu) &= \left[I-\chi^{(0)}(\mathbf{q},i\nu)(U)\right]^{-1}\chi^{(0)}(\mathbf{q},i\nu), \\
\chi^{(c)}(\mathbf{q},i\nu) &= \left[I+\chi^{(0)}(\mathbf{q},i\nu)(U)\right]^{-1}\chi^{(0)}(\mathbf{q},i\nu),
\end{aligned} \tag{4}$$

where $\chi^{(s(c))}(\mathbf{q},i\nu_n)$, $\chi^{(0)}(\mathbf{q},i\nu_n)$ and $(U)$ are $16\times16$ matrices with elements of the matrix $(U)$ to be $(U)^{\mu\nu}_{\theta\xi} = U\delta_{\mu=\nu=\theta=\xi}$.

### B. Pairing symmetry

Let's consider a cooper pair with momentum/orbital $(\mathbf{k}'t, -\mathbf{k}'s)$, which could be scattered to $(\mathbf{k}p, -\mathbf{k}q)$ by charge or spin fluctuations. In the RPA level, The effective interaction induced by

this process is as follow,

$$V_{eff}^{RPA} = \frac{1}{N} \sum_{pqst,kk'} \Gamma_{st}^{pq}(k,k') c_p^\dagger(\mathbf{k}) c_q^\dagger(-\mathbf{k}) c_s(-\mathbf{k}') c_t(\mathbf{k}'), \tag{5}$$

In the singlet channel, the effective vertex $\Gamma_{st}^{pq}(k,k')$ is given as follow,

$$\begin{aligned}\Gamma_{st}^{pq}(k,k') = (U)_{qs}^{pt} + \frac{1}{4}\left\{(U)\left[3\chi^{(s)}\left(k-k'\right) - \chi^{(c)}\left(k-k'\right)\right](U)\right\}_{qs}^{pt} + \\ \frac{1}{4}\left\{(U)\left[3\chi^{(s)}\left(k+k'\right) - \chi^{(c)}\left(k+k'\right)\right](U)\right\}_{qt}^{ps},\end{aligned} \tag{6}$$

while in the triplet channel, it is

$$\begin{aligned}\Gamma_{st}^{pq}(k,k') = -\frac{1}{4}\left\{(U)\left[\chi^{(s)}\left(k-k'\right) + \chi^{(c)}\left(k-k'\right)\right](U)\right\}_{qs}^{pt} + \\ \frac{1}{4}\left\{(U)\left[\chi^{(s)}\left(k+k'\right) + \chi^{(c)}\left(k+k'\right)\right](U)\right\}_{qt}^{ps}.\end{aligned} \tag{7}$$

Notice that the vertex $\Gamma_{st}^{pq}(k,k')$ has been symmetrized for the singlet case and anti-symmetrized for the triplet case. Generally we neglect the frequency-dependence of $\Gamma$ and replace it by $\Gamma_{st}^{pq}(k,k') \approx \Gamma_{st}^{pq}(\mathbf{k},\mathbf{k}',0)$.

Projecting the above effective interaction (5) into the two bands which cross the FS, we obtain the following low energy effective Hamiltonian for the cooper pairs near the FS,

$$V_{eff} = \frac{1}{N} \sum_{\alpha\beta,\mathbf{kk}'} V^{\alpha\beta}(\mathbf{k},\mathbf{k}') c_\alpha^\dagger(\mathbf{k}) c_\alpha^\dagger(-\mathbf{k}) c_\beta(-\mathbf{k}') c_\beta(\mathbf{k}'), \tag{8}$$

where $\alpha, \beta = 1, 2$ and $V^{\alpha\beta}(\mathbf{k},\mathbf{k}')$ is

$$V^{\alpha\beta}(\mathbf{k},\mathbf{k}') = \mathrm{Re} \sum_{pqst,\mathbf{kk}'} \Gamma_{st}^{pq}(\mathbf{k},\mathbf{k}',0) \xi_p^{\alpha,*}(\mathbf{k}) \xi_q^{\alpha,*}(-\mathbf{k}) \xi_s^{\beta}(-\mathbf{k}') \xi_t^{\beta}(\mathbf{k}'). \tag{9}$$

Here only intra-band pairing is considered for small U.

From the low energy effective Hamiltonian (8), one can obtain the following linearized gap equation[9] to determine the $T_c$ and the leading pairing symmetry of the system,

$$-\frac{1}{(2\pi)^2} \sum_\beta \oint_{FS} dk'_\parallel \frac{V^{\alpha\beta}(\mathbf{k},\mathbf{k}')}{v_F^\beta(\mathbf{k}')} \Delta_\beta(\mathbf{k}') = \lambda \Delta_\alpha(\mathbf{k}). \tag{10}$$

Here, the integration and summation is along various FS patches labelled by $\alpha$ or $\beta$. The $v_F^{\beta}(\mathbf{k}')$ is Fermi velocity at $\mathbf{k}'$ on the $\beta-$th FS patch, and $k'_{\parallel}$ represents the component along that patch. In this eigenvalue problem, the normalized eigenvector $\Delta_{\alpha}(\mathbf{k})$ represents the relative value of the gap function on the $\alpha-$th FS patches near $T_c$ determined by

$$T_c = 1.13\hbar\omega_D e^{-1/\lambda}. \tag{11}$$

The leading pairing symmetry of the system is thus determined by the largest eigenvalue $\lambda$ of Eq.(10).

## III. MORE DETAILS OF THE PAIRING SYMMETRIES OBTAINED

The $d + id'$ pairing symmetry identified here is robust against small dopings. Our RPA calculations yield that for $U = 1\ eV$, the leading pairing symmetries of the system are still degenerate $d_{x^2-y^2}$ and $d_{xy}$ doublets for both the 5% electron-doped case shown in Fig.3a and the 5% hole-doped case shown in Fig.3b although the FS topology has been modified in these cases. The two gap functions are symmetry related: they form a 2D $E_g$ representation of the $D_{3d}$ point-group of the system, and thus are exactly degenerate. While the gap function of the $d_{x^2-y^2}$ symmetry is antisymmetric about the axises $x = \pm y$ shown in the reciprocal space, that of the $d_{xy}$ (Fig.4(a)) symmetry is symmetric about them. Mean-field calculations involving the effective interaction induced by exchanging spin fluctuations always reveal $d + id'$ as the energetically favored superposition manner between the doublets.

It is interesting to note that our RPA calculations also identify a possible f-wave SC shown in Fig.4(b) to be the leading one in the triplet channel at half-filling. The gap function of this pairing changes sign with every $60^o$ rotation. It is antisymmetric about the three diagonal lines shown in the Brillouin-Zone, which are just the gap node lines. This gap function belongs to $A_{1u}$ irreducible representation of $D_{3d}$. Similarly with the $d + id'$ symmetry, this pairing also satisfies the requirement that gap nodes should avoid the FS. Positive eigenvalue $\lambda$ corresponding to this symmetry suggests finite $T_c$ of the pairing, which is nevertheless much lower than that of the $d+id'$

symmetry.

---

[1] T. Morishita, S. P. Russo, I. K. Snook, M. J. S. Spencer, K. Nishio, and M. Mikami, Phys. Rev. B **82**, 045419 (2010).

[2] B. Feng, Z. Ding, S. Meng, Y. Yao, X. He, P. Cheng, L. Chen, and K. Wu, Nano Letters **12**, 3507 (2012).

[3] X. D. Wen, T. J. Cahill, and R. Hoffmann, Chemistry **16**, 6555 (2010).

[4] T. Takimoto, T. Hotta, and K. Ueda, Phys. Rev. B **69**, 104504 (2004).

[5] K. Yada and H. Kontani, J. Phys. Soc. Jpn. **74**, 2161 (2005).

[6] K. Kubo, Phys. Rev. B **75**, 224509 (2007).

[7] I. I. Mazin, D. J. Singh, M. D. Johannes, and M. H. Du, Phys. Rev. Lett. **101**, 057003 (2008).

[8] K. Kuroki, S. Onari, R. Arita, H. Usui, Y. Tanaka, H. Kontani, and H. Aoki, Phys. Rev. Lett. **101**, 087004 (2008).

[9] S. Graser, T. A. Maier, P. J. Hirschfeld, and D. J. Scalapino, New Journal of Physics **11**, 025016 (2009).

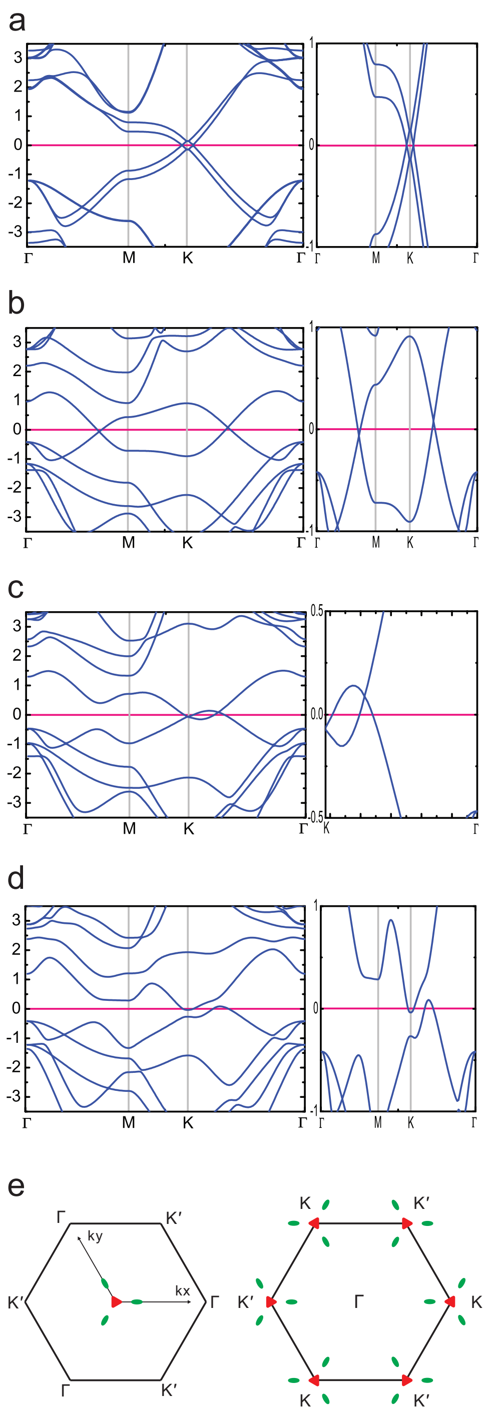


FIG. 2: **Possible band structures for the BLS. a-d**, The band structures for the AA-bb (a), AA-bt (b), AB-bt (c) and AB-bb (d) respectively. Low energy zooming in for each band is also shown. **e**, Diagrams for the FS, where red(green) region stands for electron(hole).

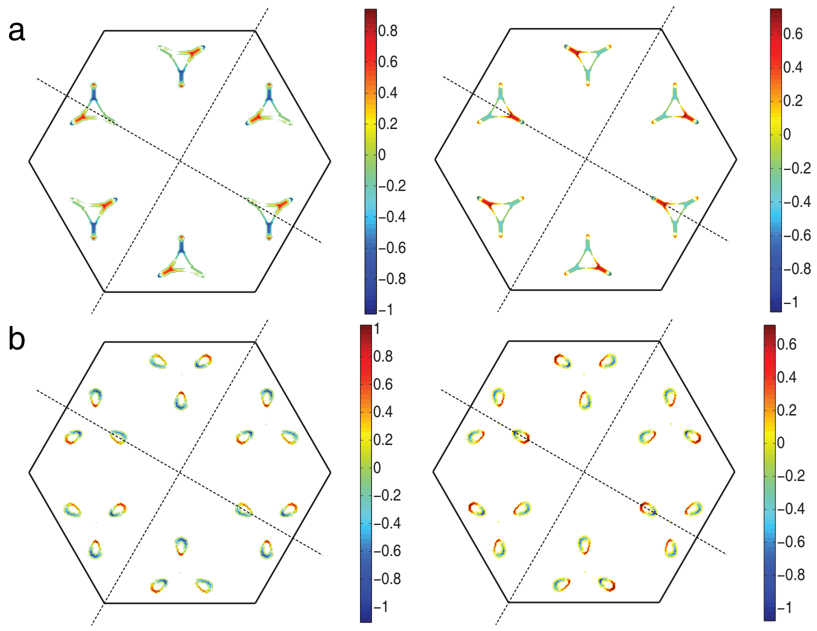


FIG. 3: **Leading pairing symmetries for the doped cases. a,b**, Leading pairing symmetries of the 5% electron-doped case (a) and 5% hole-doped case (b) for $U = 1\ eV$. In each show, the left is the $d_{x^2-y^2}$ and the right is the $d_{xy}$.

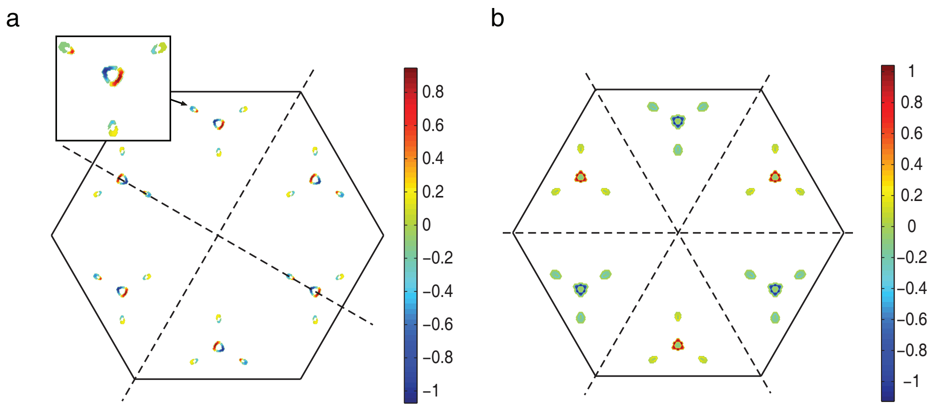


FIG. 4: **Gap function.** (a) Gap function of the $d_{xy}$ symmetry for U=1 eV, which is symmetric about the axises $x = \pm y$. Inset: zooming in the vicinity of $\mathbf{K}'$. (b) Normalized relative gap function of the f-wave pairing, obtained as the leading symmetry in the triplet channel at half-filling for U=1 eV.
